# Supplementary material for: What Do VLMs NOTICE? A Mechanistic Interpretability Pipeline for Gaussian-Noise-free Text-Image Corruption and Evaluation
Source: arXiv:2406.16320 source file (2025-02-07)
Supplement: Supplementary file 1 [file appendix.tex]

\begin{figure}[htbp]
    \centering
    \includegraphics[width=\textwidth]{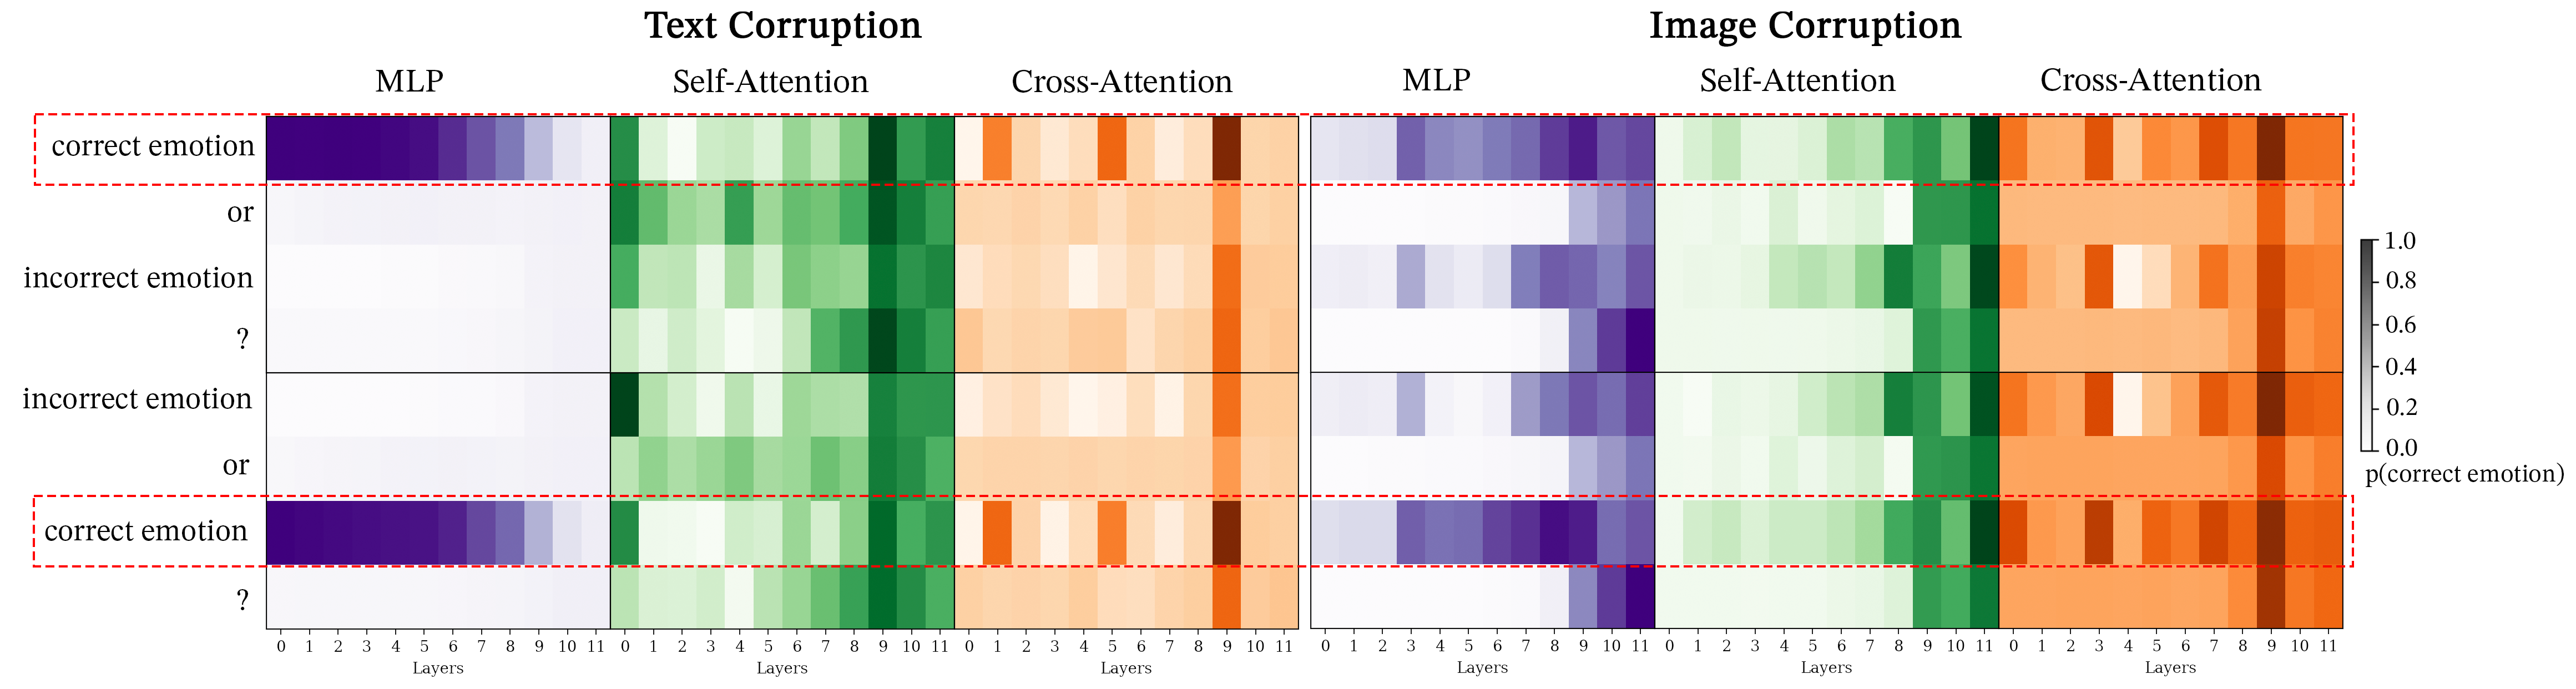}
    \caption{BLIP Emotions}
    \label{fig:blip_emotions}
\end{figure}

\begin{figure}[htbp]
    \centering
    \includegraphics[width=\textwidth]{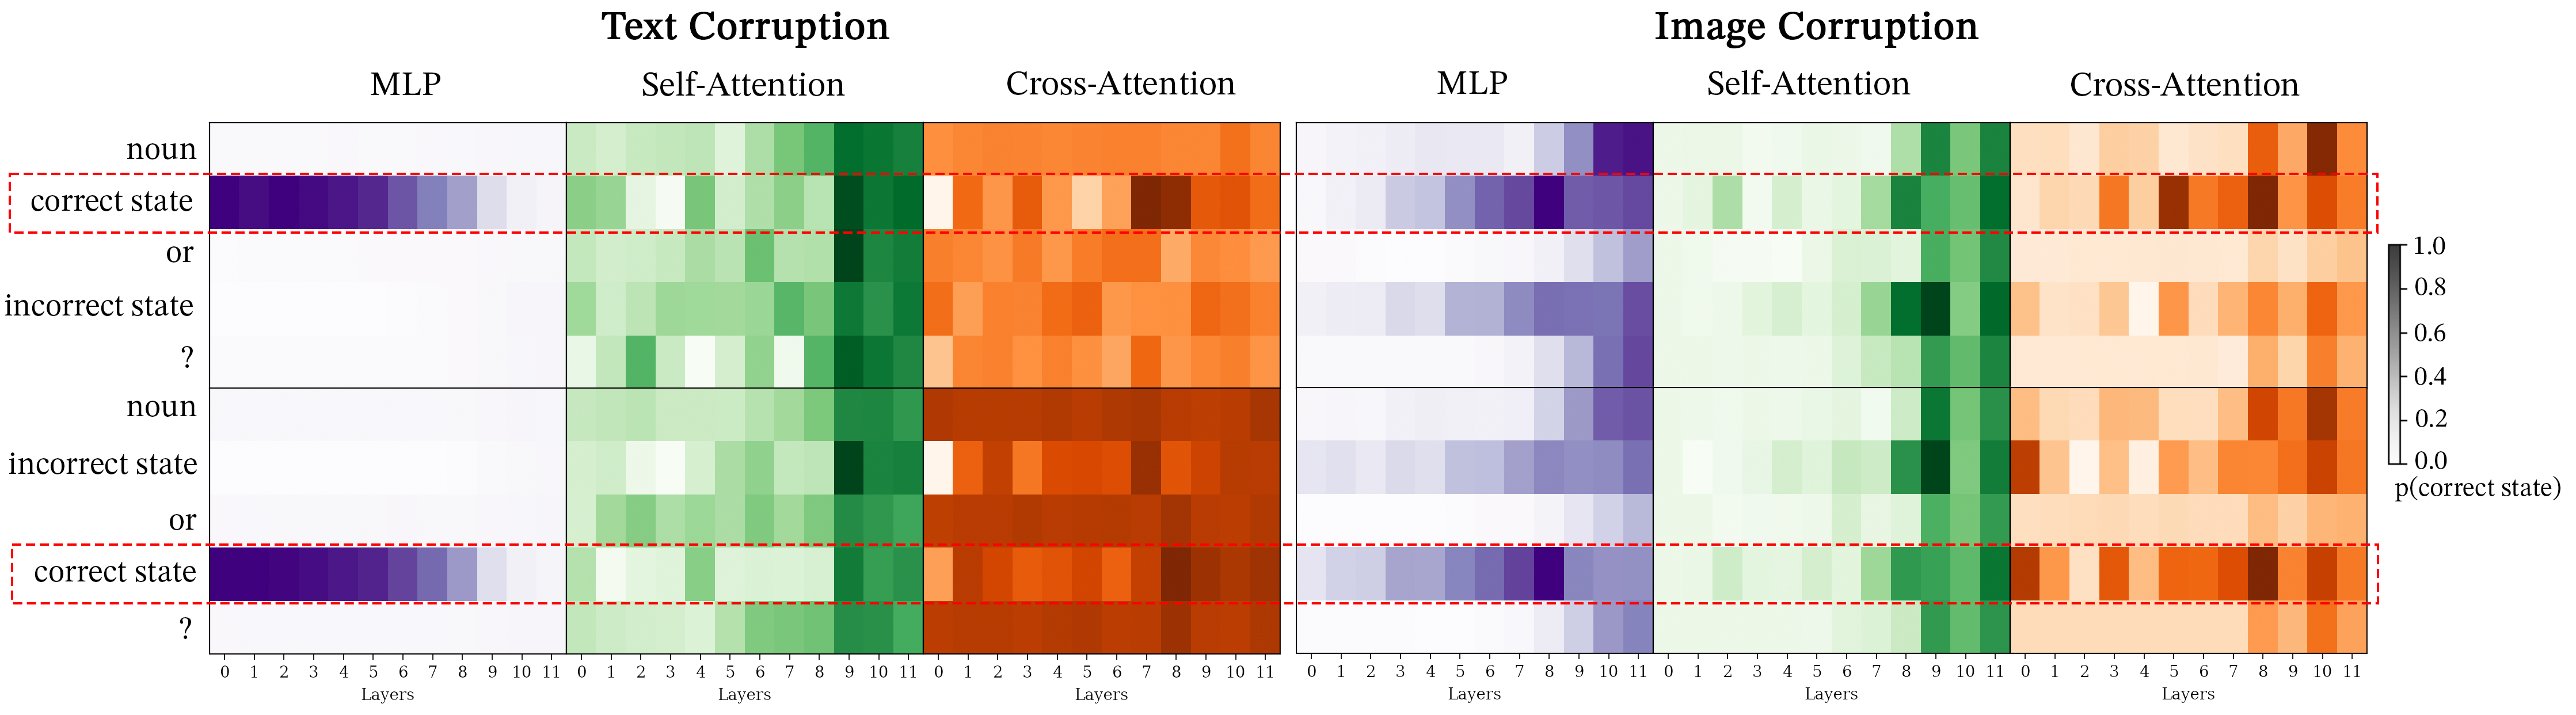}
    \caption{BLIP MIT States}
    \label{fig:blip_mit_states}
\end{figure}

\begin{figure}[htbp]
    \centering
    \includegraphics[width=\textwidth]{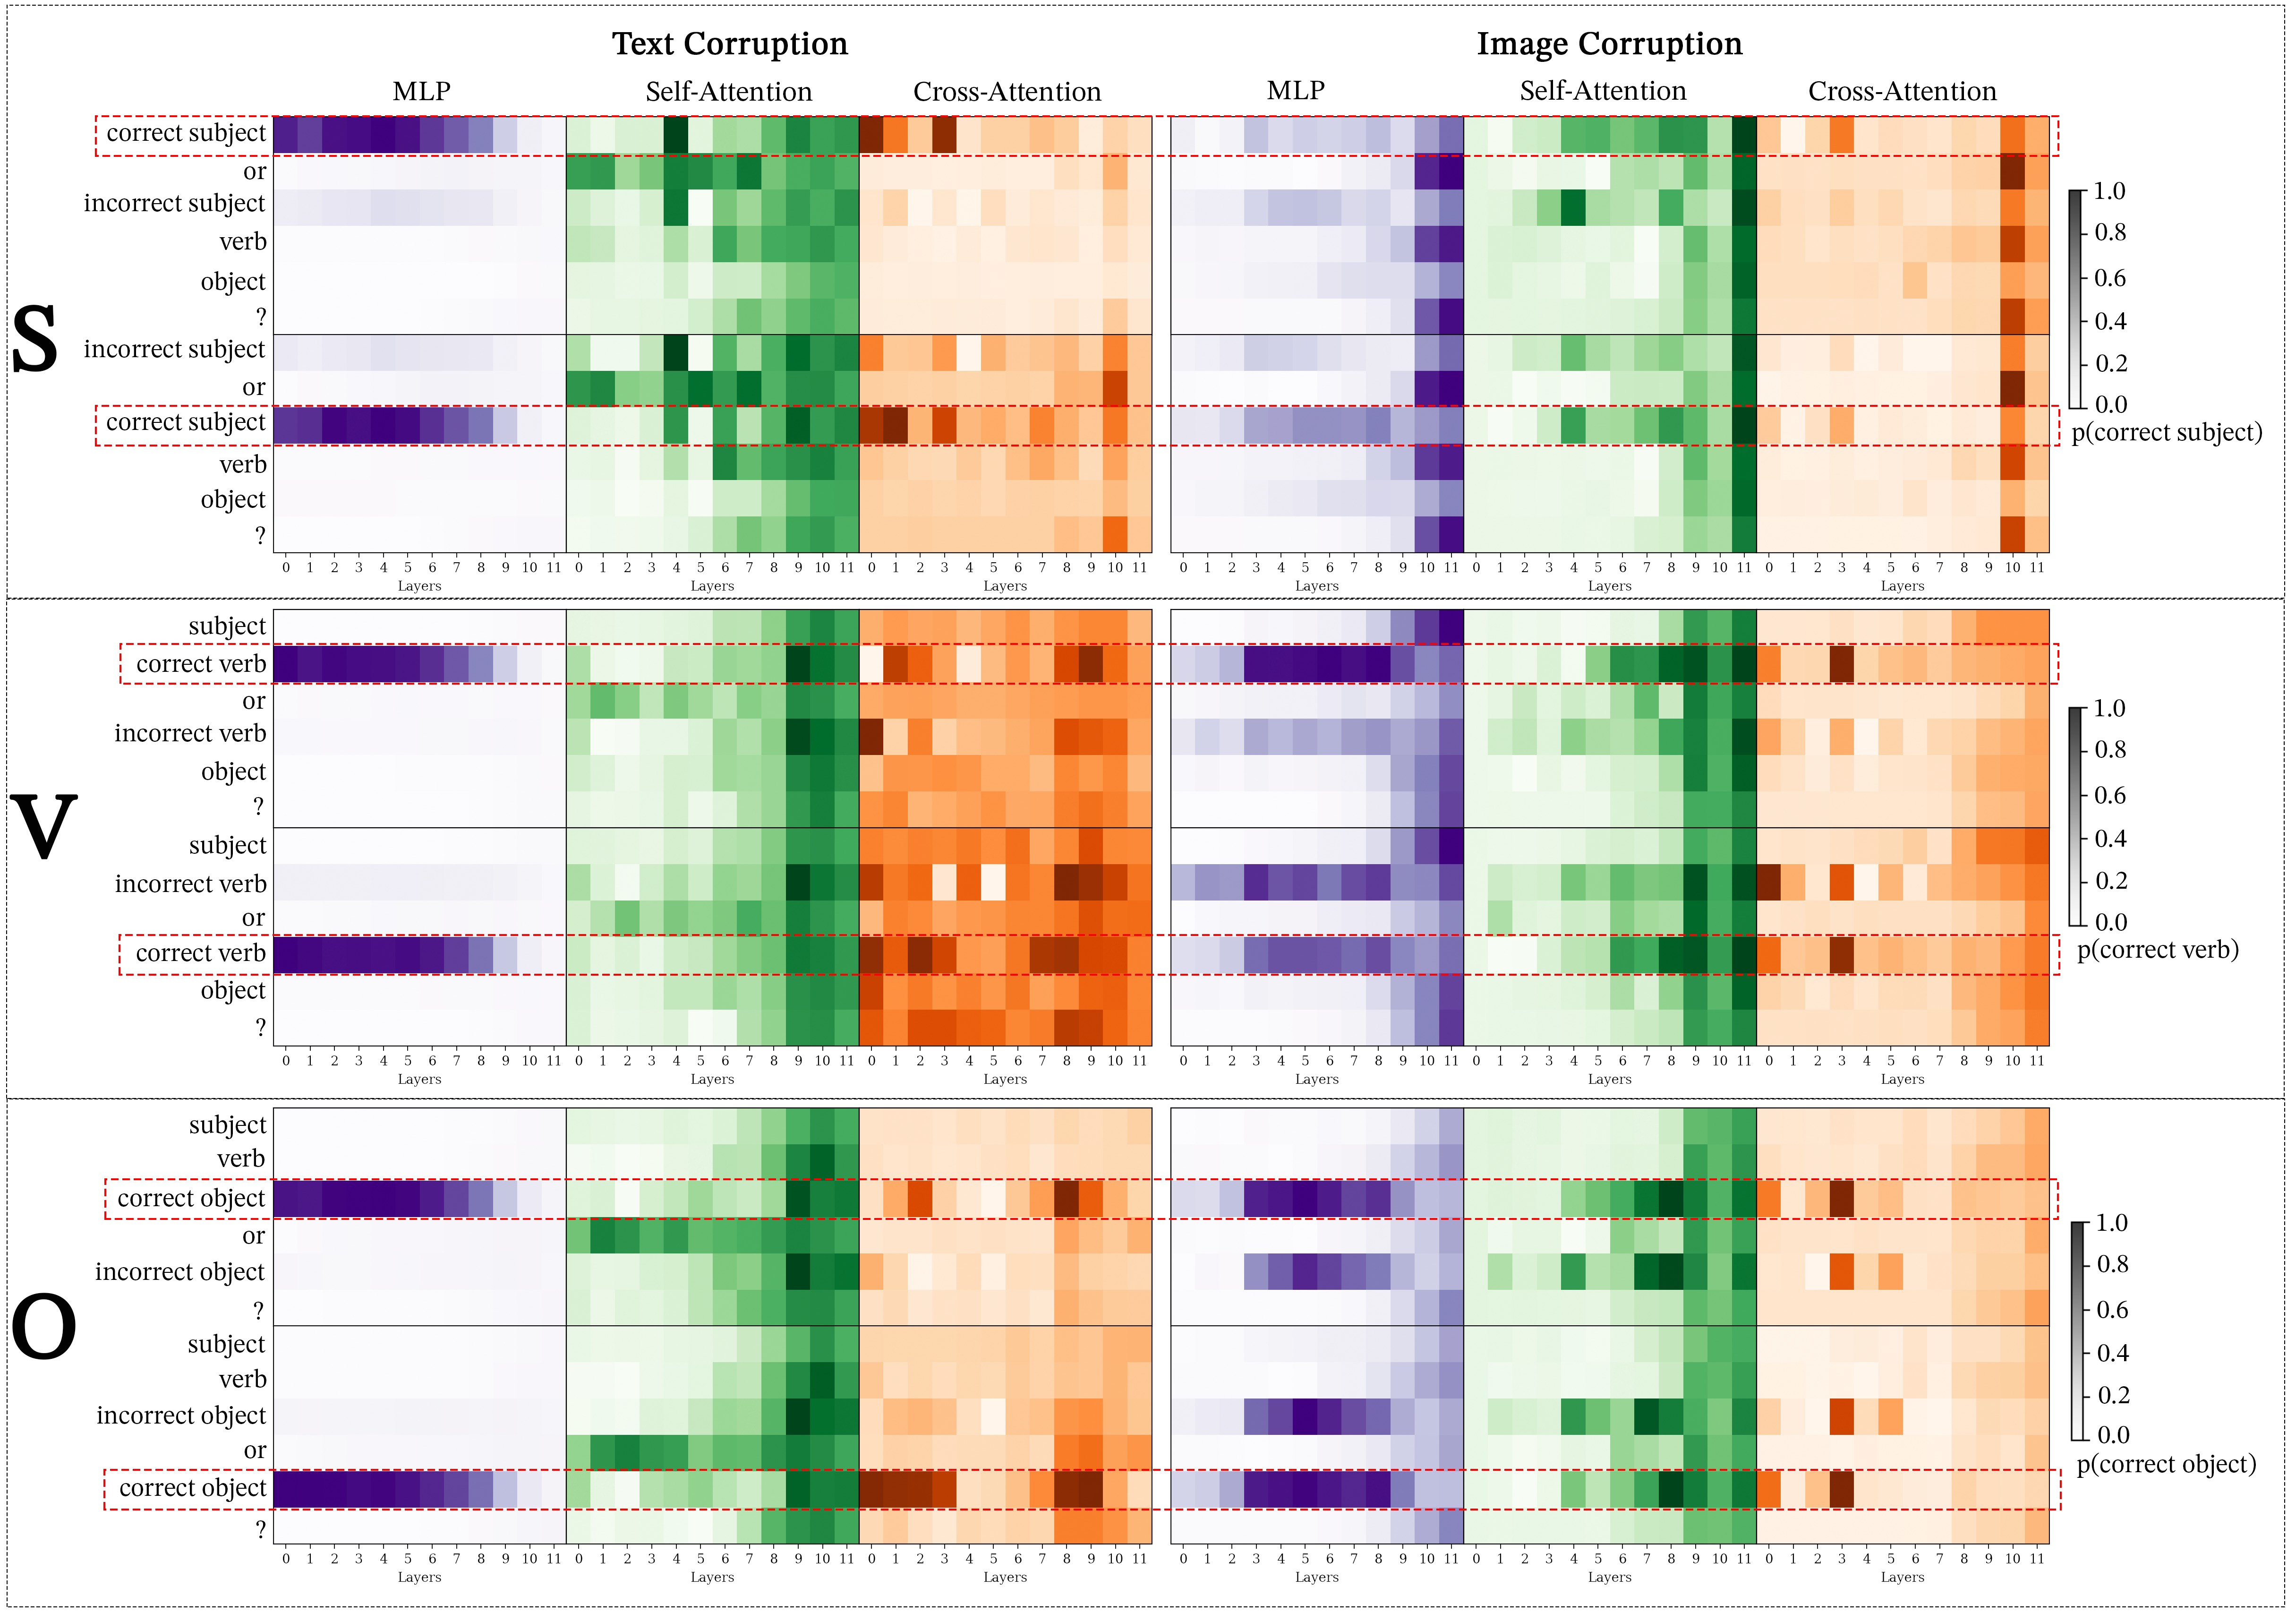}
    \caption{BLIP SVO}
    \label{fig:blip_svo}
\end{figure}

\begin{figure}[htbp]
    \centering
    \includegraphics[width=\textwidth]{BLIP2_svo_appendix.png}
    \caption{BLIP2 SVO}
    \label{fig:blip2_svo}
\end{figure}

\begin{figure}[htbp]
    \centering
    \includegraphics[width=\textwidth]{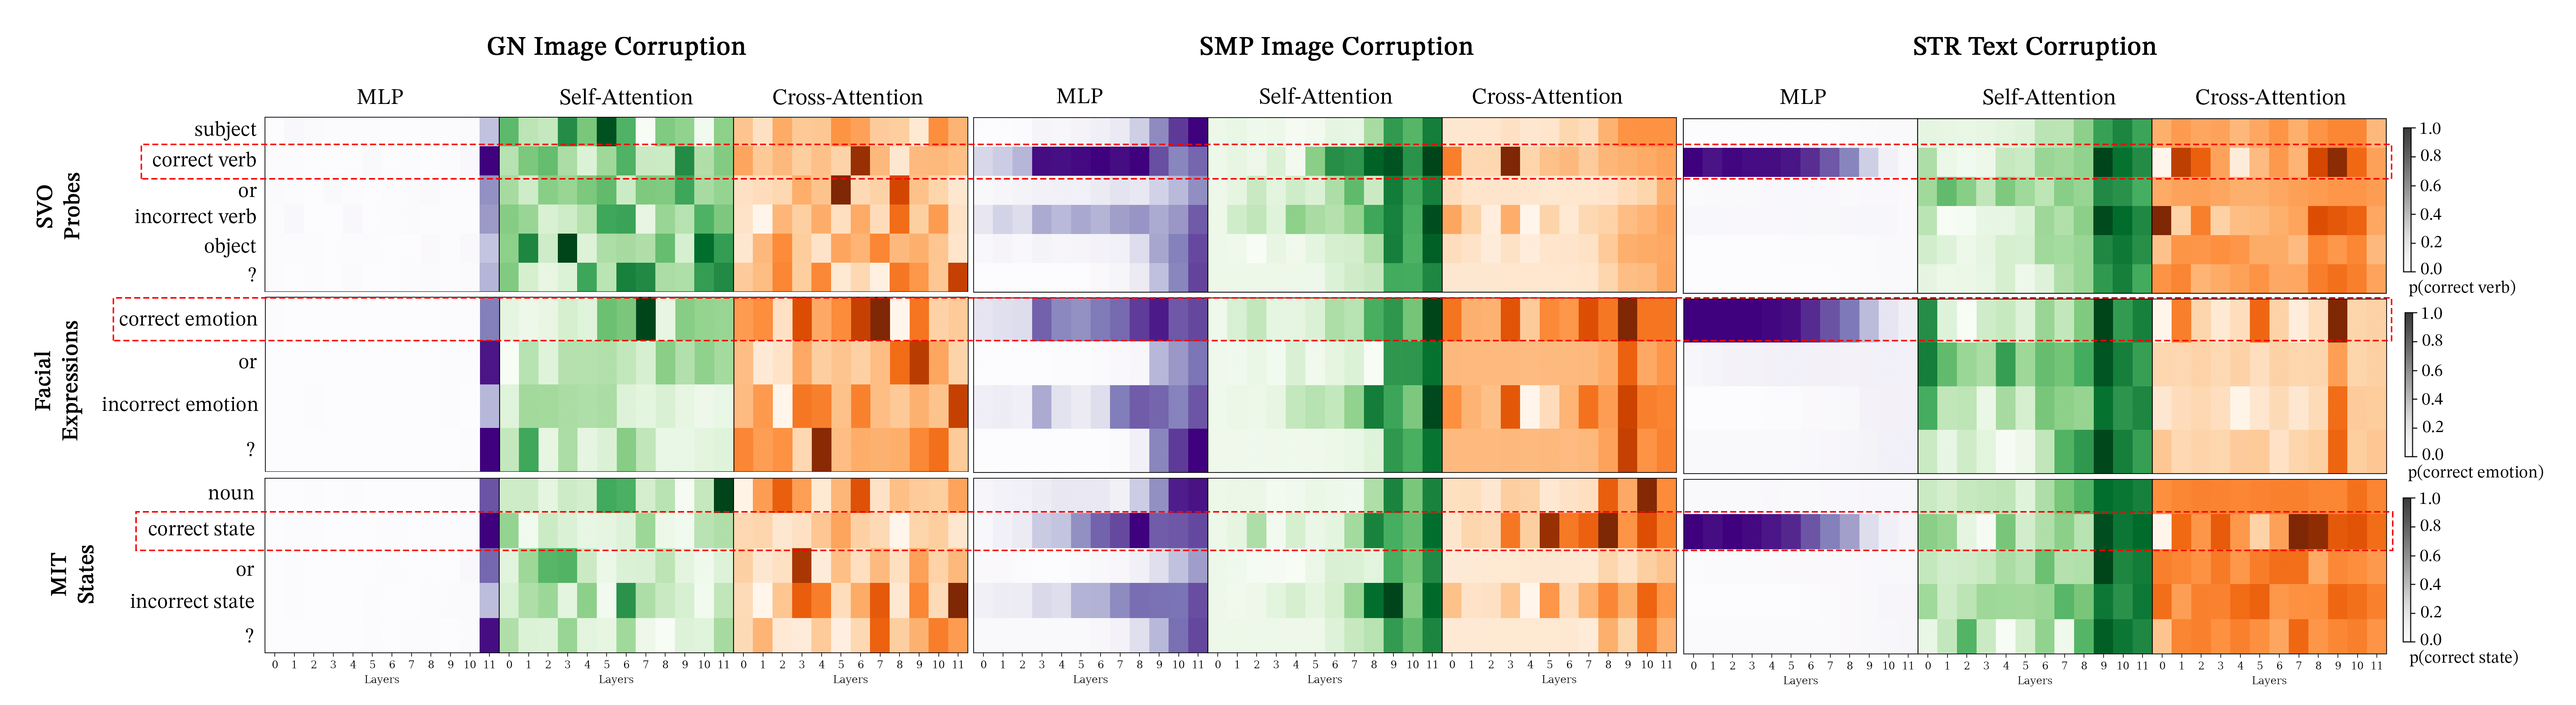}
    \caption{BLIP2 SVO}
    \label{fig:blip2_svo}
\end{figure}
